# Supplementary material for: LEMON: Localized Editing with Mesh Optimization and Neural Shaders
Source: arXiv:2409.12024 source file (2024-09-18)
Supplement: Supplementary file 1 [file Supp.pdf]

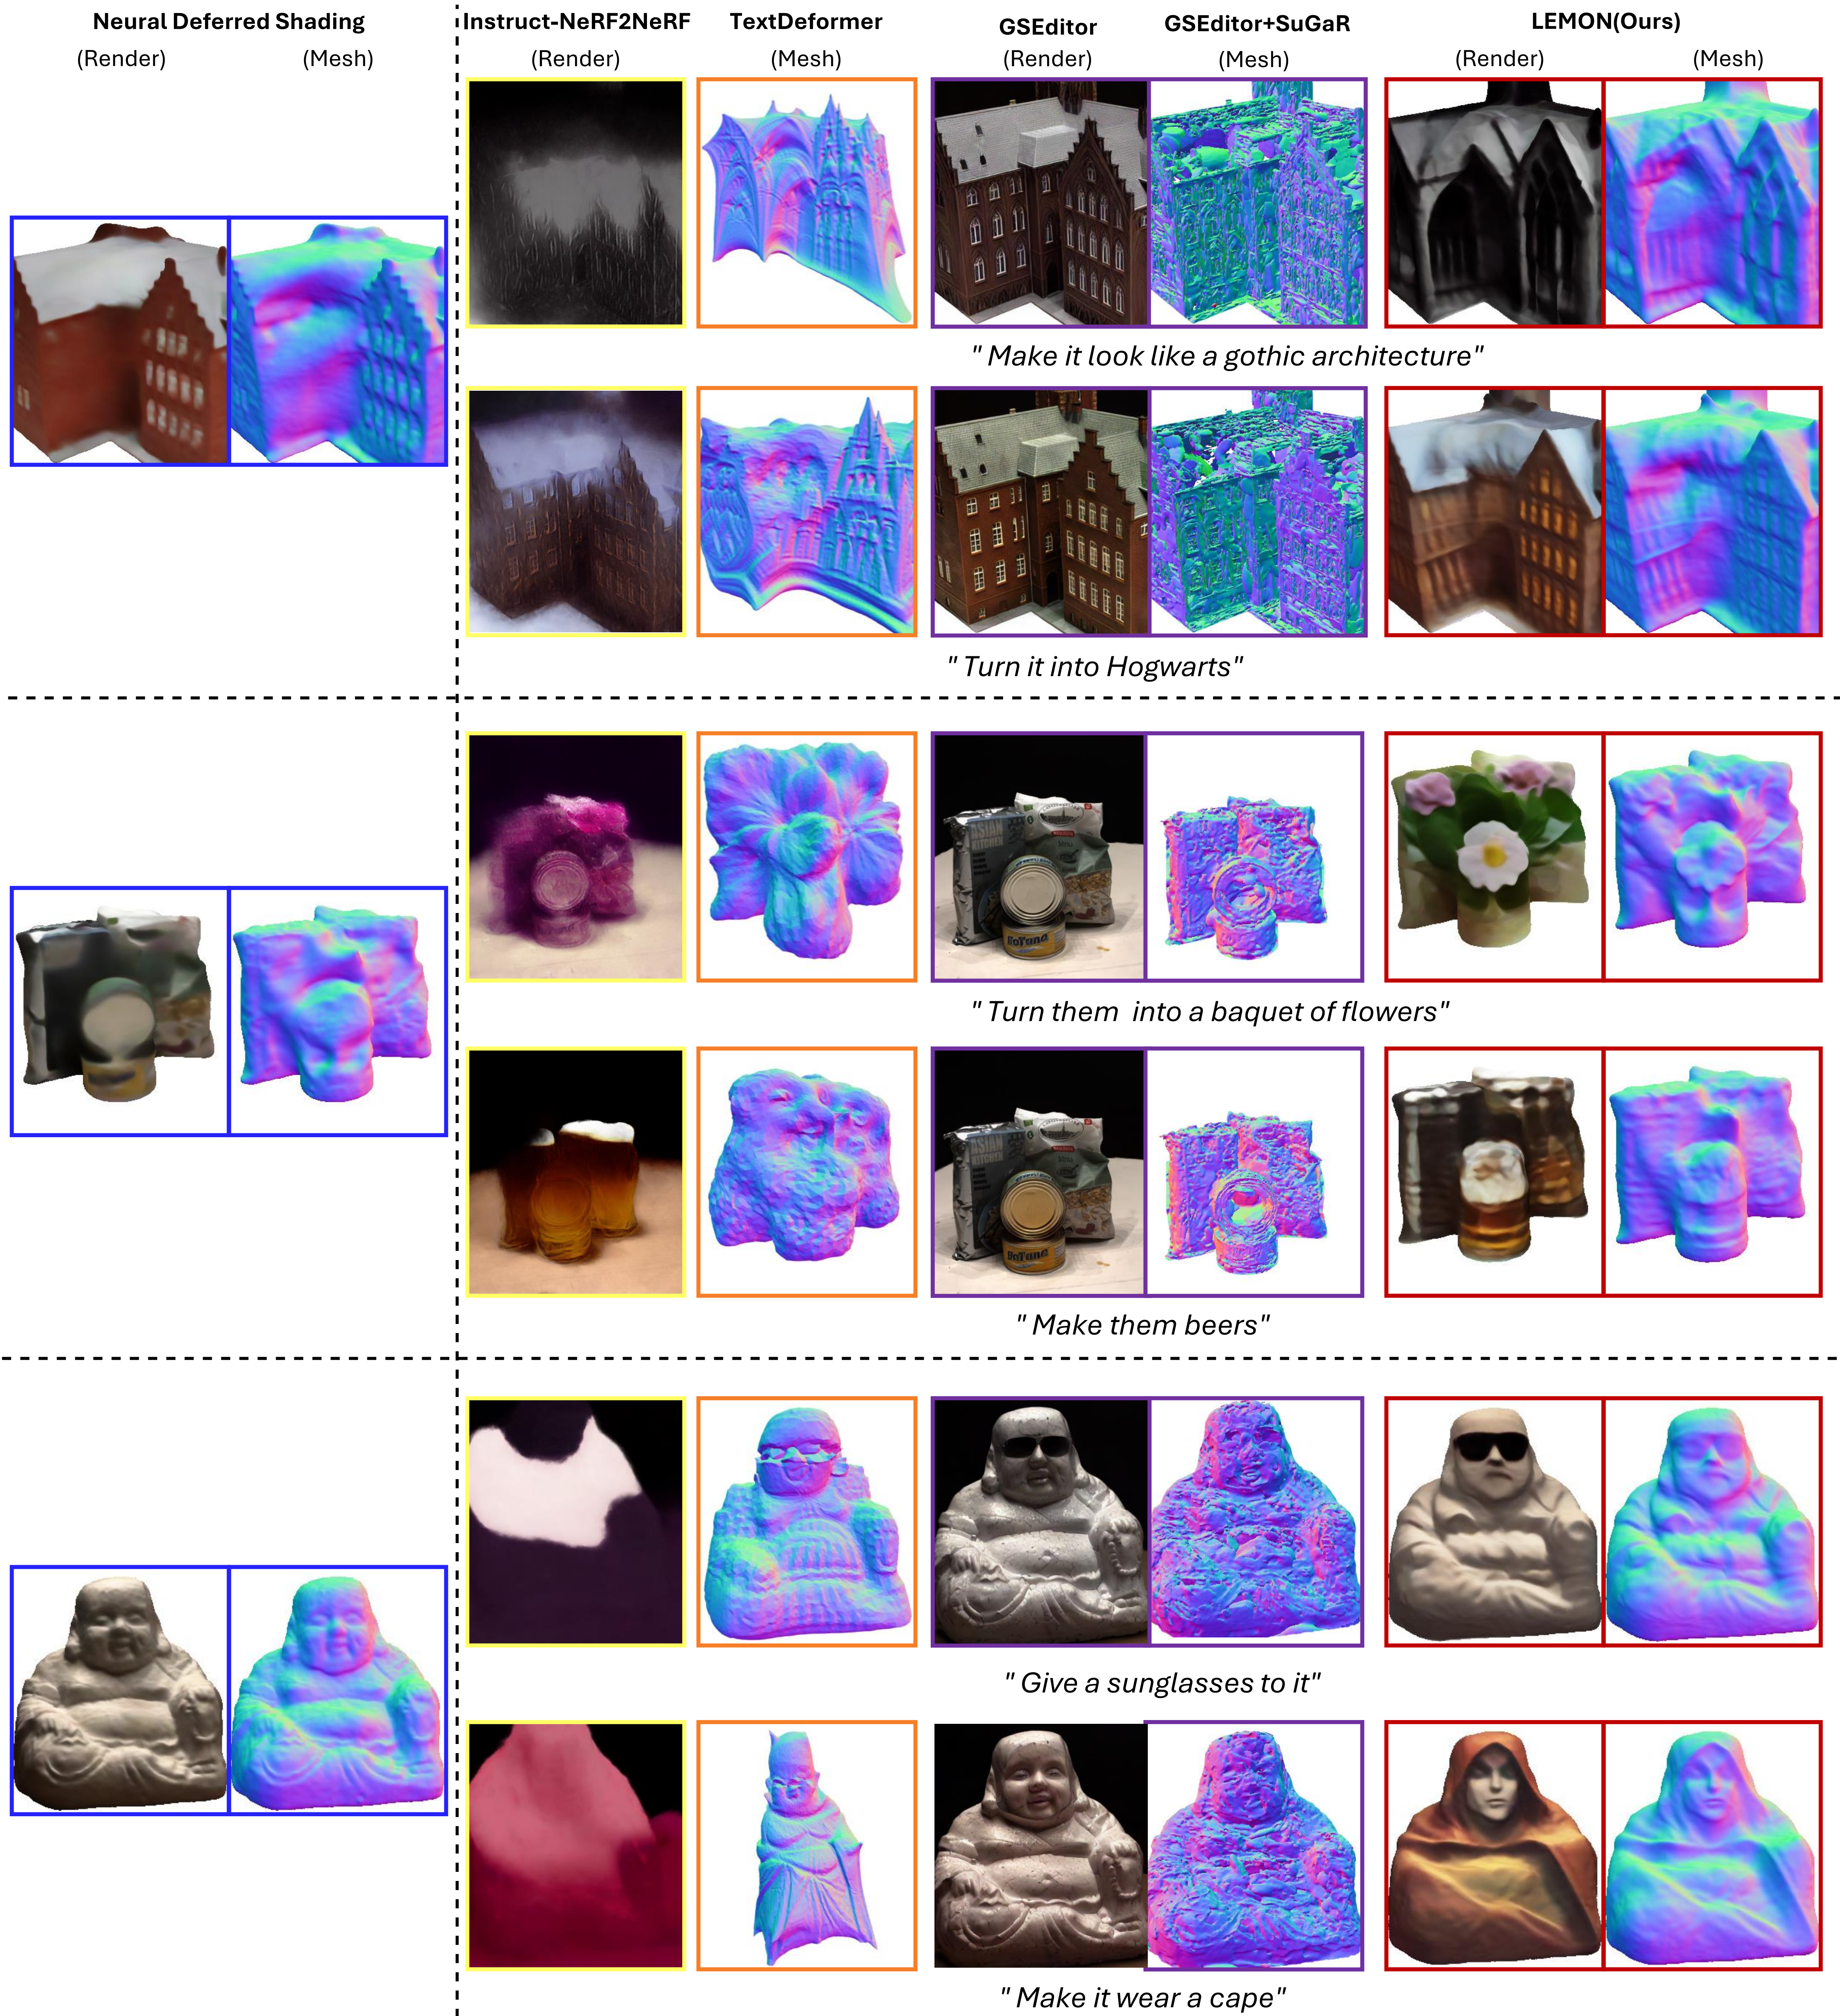
Neural Deferred Shading
(Render)
(Mesh)
Instruct-NeRF2NeRF
(Render)
TextDeformer
(Mesh)
GSEditor
(Render)
GSEditor+SuGaR
(Mesh)
LEMON(Ours)
(Render)
(Mesh)
" Make it look like a gothic architecture"
" Turn it into Hogwarts"
" Turn them into a baquet of flowers"
" Make them beers"
" Give a sunglasses to it"
" Make it wear a cape"

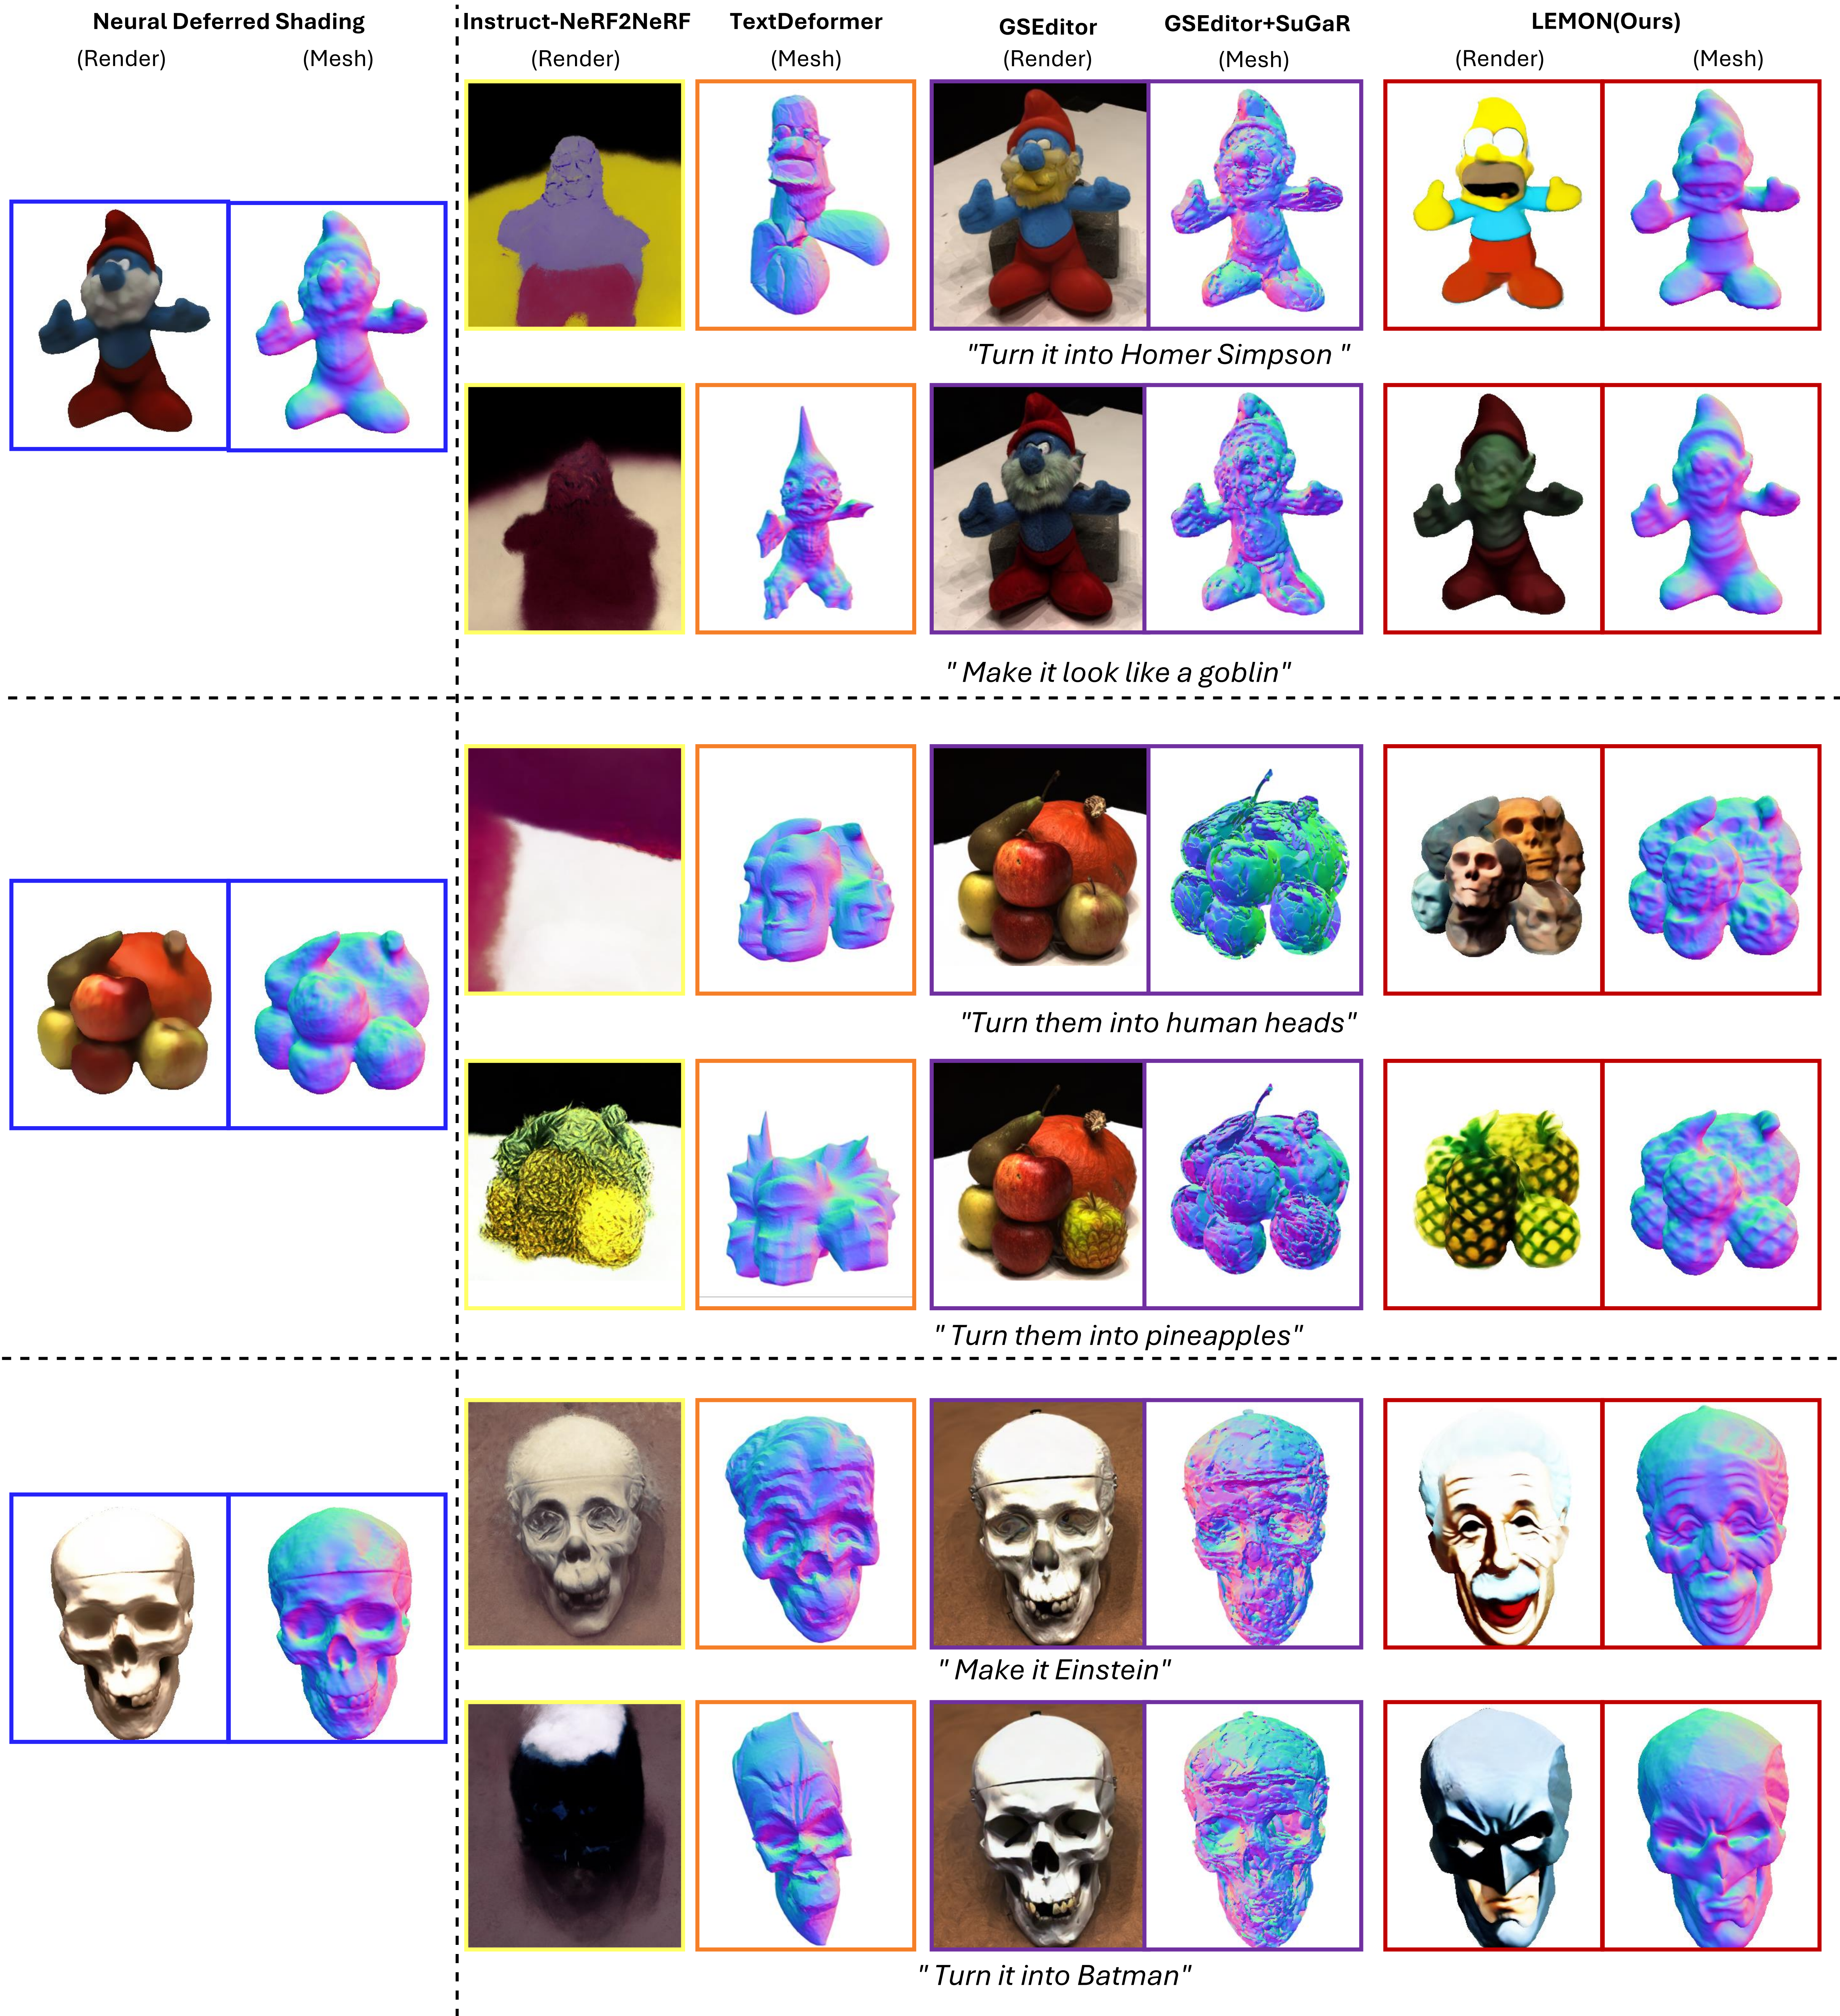
Neural Deferred Shading
(Render)
(Mesh)
Instruct-NeRF2NeRF
(Render)
TextDeformer
(Mesh)
GSEditor
(Render)
GSEditor+SuGaR
(Mesh)
LEMON(Ours)
(Render)
(Mesh)
"Turn it into Homer Simpson "
" Make it look like a goblin"
"Turn them into human heads"
" Turn them into pineapples"
" Make it Einstein"
" Turn it into Batman"

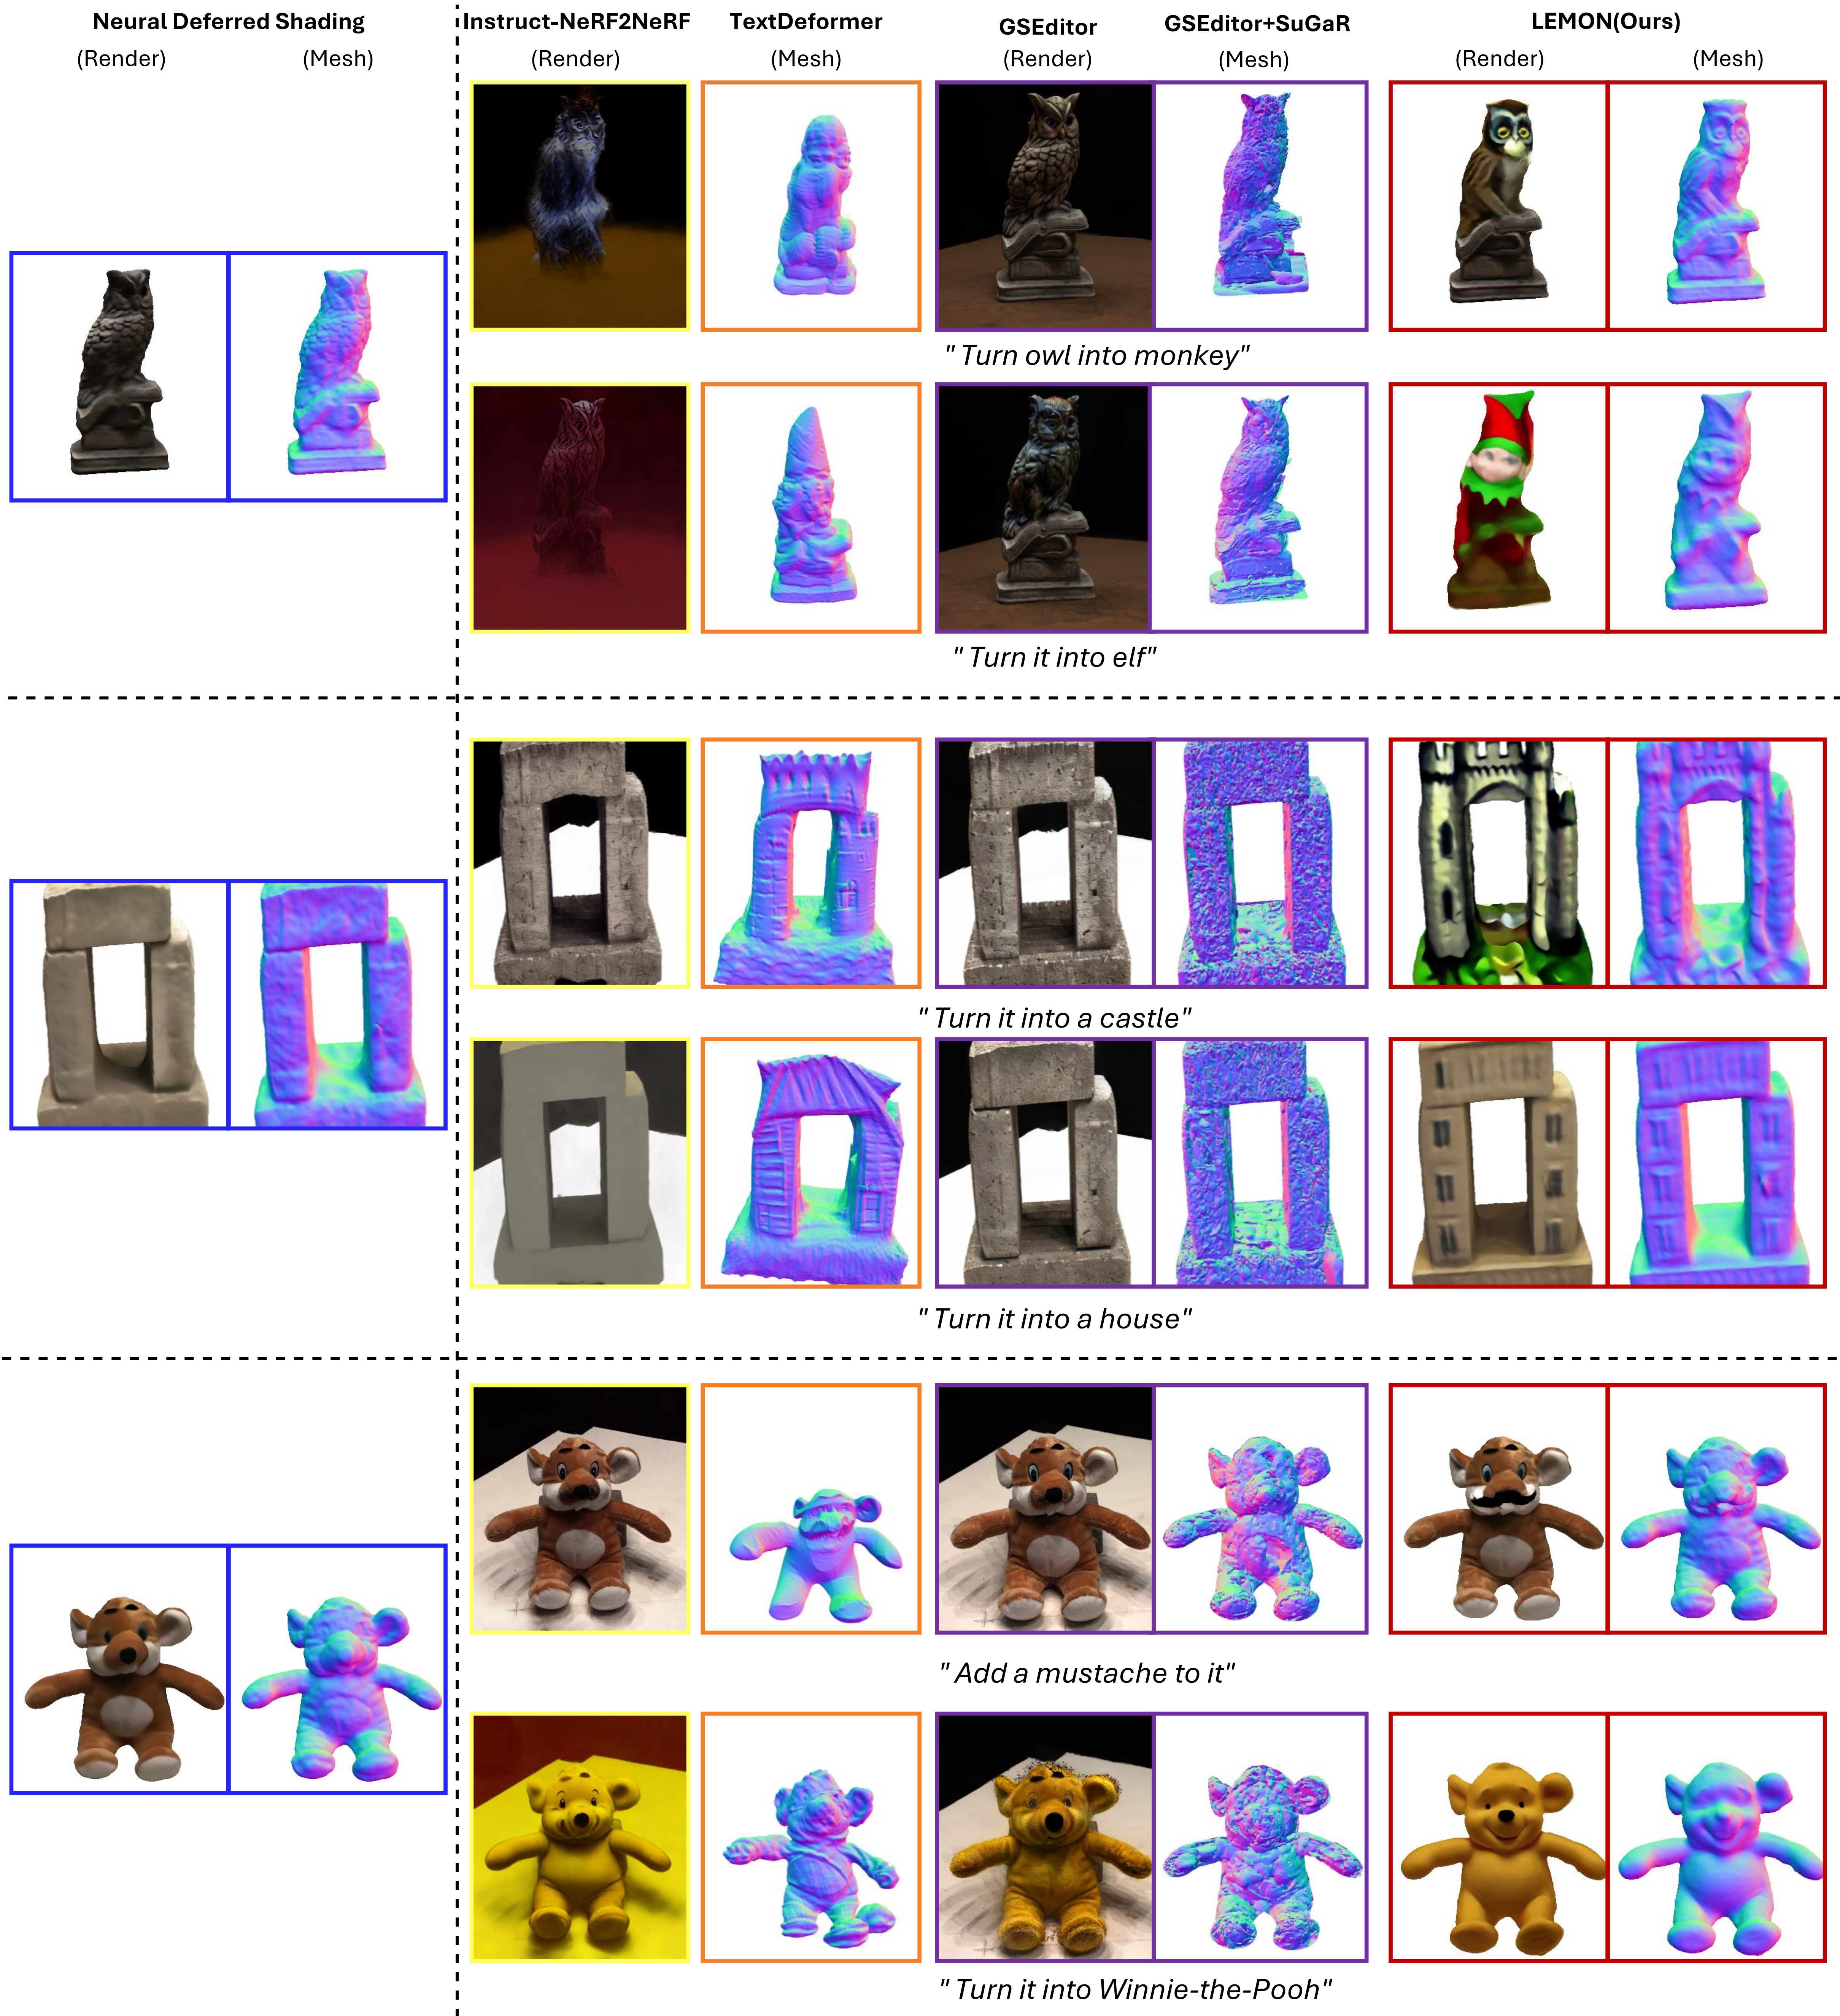

Neural Deferred Shading
(Render)
(Mesh)
Instruct-NeRF2NeRF
(Render)
TextDeformer
(Mesh)
GSEditor
(Render)
GSEditor+SuGaR
(Mesh)
LEMON(Ours)
(Render)
(Mesh)
" Turn owl into monkey"
" Turn it into elf"
" Turn it into a castle"
" Turn it into a house"
" Add a mustache to it"
" Turn it into Winnie-the-Pooh"
